# Supplementary material for: On the Convergence Speed of Spatially Coupled LDPC Ensembles
Source: arXiv:1307.3780 source file (2013-07-14)
Supplement: Supplementary file 1 [file supp-pdf.mkii.tex]

%D \module
%D   [       file=supp-pdf,
%D        version=2006.09.02, % 2004.12.16,
%D          title=\CONTEXT\ Support Macros,
%D       subtitle=\METAPOST\ to \PDF\ conversion,
%D         author=Hans Hagen \& others (see text),
%D           date=\currentdate,
%D      copyright={PRAGMA ADE \& \CONTEXT\ Development Team}]
%C
%C This module is part of the \CONTEXT\ macro||package and is
%C therefore copyrighted by \PRAGMA. See mreadme.pdf for
%C details.

\ifx\writestatus\undefined
  \immediate\write16{[Loading MPS to PDF converter (version 2006.09.02).]}
\else
  \writestatus{loading}{ConTeXt Support Macros / PDF}
\fi

%D This module is not optimized because it is used outside
%D \CONTEXT\ and we cannot forsee what interference will take
%D place. We no longer load supp-mis. I got too tired of
%D keeping track of interferences with non \CONTEXT\ usage so
%D I moved the necessary code in here and use a derived version
%D in \CONTEXT. When I have the time I will clean up some of the
%D code that is of no use for non||\CONTEXT\ users.

\ifx\contextversion\undefined

    \chardef\mptopdfstoredatcode\catcode`\@

    \catcode\string`@=11

    \def\unprotect
      {\let\@@mpstopdf@@unprotect   \unprotect
       \let\@@mpstopdf@@protect     \protect
       \edef\protect
         {\noexpand \let \noexpand \protect   \noexpand \@@mpstopdf@@protect
          \noexpand \let \noexpand \unprotect \noexpand \@@mpstopdf@@unprotect
          % context specific
          \catcode\string`\noexpand @=\the\catcode\string`@
          \catcode\string`\noexpand !=\the\catcode\string`!
          \catcode\string`\noexpand ?=\the\catcode\string`?
          % latex specific
          \catcode\string`\noexpand /=\the\catcode\string`/
          \catcode\string`\noexpand -=\the\catcode\string`-
          \catcode\string`\noexpand :=\the\catcode\string`:
          \catcode\string`\noexpand ;=\the\catcode\string`;
          \catcode\string`\noexpand "=\the\catcode\string`"
          \catcode\string`\noexpand <=\the\catcode\string`<
          \catcode\string`\noexpand >=\the\catcode\string`>
          \catcode\string`\noexpand `=\the\catcode\string``}
      \catcode\string`@=11 \catcode\string`!=11 \catcode\string`?=11
      \catcode\string`/=12 \catcode\string`-=12
      \catcode\string`:=12 \catcode\string`;=12
      \catcode\string`>=12 \catcode\string`<=12
      \catcode\string`"=12 \catcode\string``=12 }

    \def\defineMPtoPDFfallbacks
      {% shortcuts
       \chardef\@@escape      0
       \chardef\@@begingroup  1
       \chardef\@@endgroup    2
       \chardef\@@endofline   5
       \chardef\@@ignore      9
       \chardef\@@space      10
       \chardef\@@letter     11
       \chardef\@@other      12
       \chardef\@@active     13
       \chardef\@@comment    14
       % placeholders
       \ifx\withoutpt         \undefined \let\withoutpt         \@@mptopdf@@withoutpt          \fi
       \ifx\twodigitrounding  \undefined \let\twodigitrounding  \@@mptopdf@@twodigitrounding   \fi
       \ifx\forgetall         \undefined \let\forgetall         \@@mptopdf@@forgetall          \fi
       \ifx\uncatcodespecials \undefined \let\uncatcodespecials \@@mptopdf@@uncatcodespecials  \fi
       \ifx\setnaturalcatcodes\undefined \let\setnaturalcatcodes\@@mptopdf@@setnaturalcatcodes \fi
       \ifx\dospecials        \undefined \let\dospecials        \@@mptopdf@@dospecials         \fi}

    \def\@@mptopdf@@forgetall
      {\parskip0pt\leftskip0pt\parindent0pt\everypar{}}

    \def\@@mptopdf@@twodigitrounding#1%
      {#1}%

    \def\@@mptopdf@@uncatcodespecials
      {\def\do##1{\catcode`##1=\@@other}\dospecials
       \catcode`\   =\@@space
       \catcode`\^^L=\@@ignore
       \catcode`\^^M=\@@endofline
       \catcode`\^^?=\@@ignore}

    \def\@@mptopdf@@setnaturalcatcodes
      {\catcode`\!=\@@other \catcode`\?=\@@other \catcode`\@=\@@other
       \catcode`\#=\@@other \catcode`\&=\@@other \catcode`\|=\@@other
       \catcode`\$=\@@other \catcode`\^=\@@other \catcode`\_=\@@other
       \catcode`\*=\@@other \catcode`\/=\@@other
       \catcode`\-=\@@other \catcode`+=\@@other
       \catcode`\==\@@other \catcode`\<=\@@other \catcode`\>=\@@other
       \catcode`\"=\@@other \catcode`\'=\@@other \catcode`\`=\@@other
       \catcode`\:=\@@other \catcode`\;=\@@other
       \catcode`\,=\@@other \catcode`\.=\@@other \catcode`\~=\@@other
       \catcode`\(=\@@other \catcode`\)=\@@other
       \catcode`\{=\@@other \catcode`\}=\@@other
       \catcode`\\=\@@other \catcode`\%=\@@other}

    \def\@@mptopdf@@dospecials
      {\do\ \do\\\do\{\do\}\do\$%
       \do\#\do\^\do\_\do\&\do\%%
       \do\~\do\^^A\do\^^K}

    {
        \catcode`\.=12
        \catcode`\p=12
        \catcode`\t=12
        \gdef\@@MPTOPDF@@WITHOUTPT#1pt{#1}
    }

    \def\@@mptopdf@@withoutpt#1%
      {\expandafter\@@MPTOPDF@@WITHOUTPT#1}

%     \def\@@mptopdf@@newabove#1#2% \dimen \name
%       {#1#2%
%        \ifnum\expandafter\gobblesixarguments\meaning#2>20\else
%          \expandafter\@@mptopdf@@newabove\expandafter#1\expandafter#2%
%        \fi}

    \def\@@mptopdf@@stripnewabove#1%
      {\ifnum10<9#1 #1\else\expandafter\@@mptopdf@@stripnewabove\fi}%

    \def\@@mptopdf@@newabove\csname#1\endcsname#2% \dimen \name
      {\csname#1\endcsname#2%
       \ifnum\expandafter\@@mptopdf@@stripnewabove\meaning#2>20\else
         \@@mptopdf@@newabove\csname#1\endcsname#2%
       \fi}

    \@@mptopdf@@newabove \csname newcount\endcsname \scratchcounter
    \@@mptopdf@@newabove \csname newdimen\endcsname \scratchdimen
                         \csname   newbox\endcsname \scratchbox

    \expandafter \newif \csname ifdone\endcsname

    \catcode`\@=\mptopdfstoredatcode

\else

    \let\defineMPtoPDFfallbacks\relax

\fi

%D These macros are written as generic as possible. Some
%D general support macro's are loaded from a small module
%D especially made for non \CONTEXT\ use. In this module I
%D use a matrix transformation macro written by Tanmoy
%D Bhattacharya. Thanks to extensive testing by Sebastian
%D Ratz I was able to complete this module within reasonable
%D time. This module has support for \METAPOST\ extensions
%D built in.
%D
%D Daniel H. Luecking came up with a better (more precise)
%D transformation method. You can recognize his comment by
%D his initials. (We keep the old code around because it's a
%D nice illustration on how a module like this evolves.)

%D Beware, we cannot use \type{\zeropoint} here since it may be
%D defined in the range \type{\dimen0} - 20 which we happen to use
%D as scratch registers; inside context we may consider
%D using dedicated registers.

%D This module handles some \PDF\ conversion and insertions
%D topics. By default, the macros use the \PDFTEX\ primitive
%D \type{\pdfliteral} when available. Since \PDFTEX\ is now the
%D default engine for \TEX\ distributions, we need a more complex
%D test.

\unprotect

\ifx\PDFcode\undefined
  \ifx\pdfliteral\undefined
    \def\PDFcode#1{\special{PDF: #1}}
  \else\ifx\pdfoutput\undefined
    \def\PDFcode#1{\special{PDF: #1}}
  \else\ifcase\pdfoutput
    \def\PDFcode#1{\special{PDF: #1}}
  \else % pdftex as well as in pdf mode
    \let\PDFcode\pdfliteral
  \fi\fi\fi
\else
  % we probably use context
\fi

%D First we define a handy constant:

\bgroup \defineMPtoPDFfallbacks \catcode`\%=\@@other \xdef\letterpercent{\string%} \egroup

%D \macros
%D   {pdfimage,pdfimages,pdfclippedimage}
%D
%D Starting with pdftex version 14, images are included more
%D natural to the form embedding. This enables alternative
%D images to be embedded.
%D
%D \starttyping
%D \pdfimage  <optional dimensions> {file}
%D \pdfimages <optional dimensions> {high res file} {low res file}
%D \stoptyping
%D
%D The first one replaces the pre||version||14 original,
%D while the latter provides alternative images.
%D
%D The next macro is dedicated to Maarten Gelderman, who
%D needed to paste prepared \PDF\ pages into conference
%D proceedings.
%D
%D \starttyping
%D \pdfclippedimage <optional dimensions> {file} {l} {r} {t} {b}
%D \stoptyping

\ifx\pdftexversion\undefined \else \ifnum\pdftexversion>13

  \def\pdfimage#1#%
    {\dopdfimage{#1}}

  \def\dopdfimage#1#2%
    {\immediate\pdfximage#1{#2}%
     \pdfrefximage\pdflastximage}

  \def\pdfimages#1#%
    {\dopdfimages{#1}}

  \def\dopdfimages#1#2#3%
    {\immediate\pdfximage#1{#2}%
     \immediate\pdfobj{[ << /Image \the\pdflastximage\space0 R /DefaultForPrinting true >> ]}%
     \immediate\pdfximage#1 attr {/Alternates \the\pdflastobj\space0 R}{#3}%
     \pdfrefximage\pdflastximage}

  \def\pdfclippedimage#1#% specs {file}{left}{right}{top}{bottom}
    {\dopdfclippedimage{#1}}

  \def\dopdfclippedimage#1#2#3#4#5#6%
    {\bgroup
     \pdfximage#1{#2}%
     \setbox\scratchbox\hbox
       {\pdfrefximage\pdflastximage}%
     \hsize\wd\scratchbox
     \advance\hsize -#3
     \advance\hsize -#4
     \vsize\ht\scratchbox
     \advance\vsize -#5
     \advance\vsize -#6
     \setbox\scratchbox\vbox to \vsize
       {\vskip-#5\hbox to \hsize{\hskip-#3\box\scratchbox\hss}}%
     \pdfxform\scratchbox
     \pdfrefxform\pdflastxform
     \egroup}

\fi \fi

%D If you want to save a few hash entries, you may prefer the
%D less readable alternatives, like:
%D
%D \starttyping
%D \def\pdfimage#1#% This one is less readable but needs no additional
%D   {\bgroup      % hash entry for the second stage macro.
%D    \def\pdfimage##1%
%D      {\immediate\pdfximage##1{#2}%
%D       \pdfrefximage\pdflastximage\egroup}}
%D \stoptyping

%D For old times sake we provide a few aliases. These will be
%D removed some day.

\ifx\pdftexversion\undefined \else \ifnum\pdftexversion>13

  \let\pdfform    =\pdfxform
  \let\pdflastform=\pdflastxform
  \let\pdfrefform =\pdfrefxform

\fi \fi

%D The main conversion macro wraps the \PDF\ codes in a box
%D that is output as an object. The graphics are embedded
%D in~\type{q} and~\type{Q} and are scaled and positioned using
%D one transform call (\type{cm}). This saves some additional
%D scaling.

%D \macros
%D   {convertMPtoPDF}
%D
%D The next set of macros implements \METAPOST\ to \PDF\
%D conversion. Because we want to test as fast as possible, we
%D first define the \POSTSCRIPT\ operators that \METAPOST\
%D uses. We don't define irrelevant ones, because these are
%D skipped anyway.

%D The converter can be made a bit faster by replacing the
%D two test macros (the ones with the many \type {\if's}) by
%D a call to named branch macros (something \typ {\getvalue
%D {xPSmoveto}}. For everyday documents with relatively
%D small graphics the gain in speed can be neglected.

\def \PScurveto          {curveto}
\def \PSlineto           {lineto}
\def \PSmoveto           {moveto}
\def \PSshowpage         {showpage}
\def \PSnewpath          {newpath}
\def \PSfshow            {fshow}
\def \PSclosepath        {closepath}
\def \PSfill             {fill}
\def \PSstroke           {stroke}
\def \PSclip             {clip}
\def \PSrlineto          {rlineto}
\def \PSsetlinejoin      {setlinejoin}
\def \PSsetlinecap       {setlinecap}
\def \PSsetmiterlimit    {setmiterlimit}
\def \PSsetgray          {setgray}
\def \PSsetrgbcolor      {setrgbcolor}
\def \PSsetcmykcolor     {setcmykcolor}
\def \PSsetdash          {setdash}
\def \PSgsave            {gsave}
\def \PSgrestore         {grestore}
\def \PStranslate        {translate}
\def \PSscale            {scale}
\def \PSconcat           {concat}
\def \PSdtransform       {dtransform}
\def \PSsetlinewidth     {setlinewidth}
\def \PSpop              {pop}

\def \PSnfont            {nfont}    % was needed for TUG98 proceedings
\def \PSspecial          {special}  % extensions to MetaPost

%D A previous version set \type {%} to ignore, which
%D simplified the following definitions. At the start of
%D conversion the percent character was made active again.
%D Because the whole graphic is one paragraph (there are no
%D empty lines) this does not give the desired effect. This
%D went unnoticed untill Scott Pakin sent me a test file
%D percent characters in a string. So, from now on we have
%D to prefix the following strings with percentages.

%D Some day I'll figure out a better solution (line by line reading
%D using \ETEX).

\edef \PSBoundingBox      {\letterpercent\letterpercent BoundingBox:}
\edef \PSHiResBoundingBox {\letterpercent\letterpercent HiResBoundingBox:}
\edef \PSExactBoundingBox {\letterpercent\letterpercent ExactBoundingBox:}
\edef \PSMetaPostSpecial  {\letterpercent\letterpercent MetaPostSpecial:}
\edef \PSMetaPostSpecials {\letterpercent\letterpercent MetaPostSpecials:}
\edef \PSPage             {\letterpercent\letterpercent Page:}
\edef \PSBeginProlog      {\letterpercent\letterpercent BeginProlog}
\edef \PSEndProlog        {\letterpercent\letterpercent EndProlog}
\edef \PSEof              {\letterpercent\letterpercent EOF}

%D By the way, the \type {setcmykcolor} operator is not
%D output by \METAPOST\ but can result from converting the
%D \cap{RGB} color specifications, as implemented in
%D \type{supp-mps}.

%D In \POSTSCRIPT\ arguments precede the operators. Due to the
%D fact that in some translations we need access to those
%D arguments, and also because sometimes we have to skip them,
%D we stack them up. The stack is one||dimensional for non path
%D operators and two||dimensional for operators inside a path.
%D This is because we have to save the whole path for
%D (optional) postprocessing. Values are pushed onto the stack
%D by:
%D
%D \starttyping
%D \setMPargument {value}
%D \stoptyping
%D
%D They can be retrieved by the short named macros:
%D
%D \starttyping
%D \gMPa {number}
%D \gMPs {number}
%D \stoptyping
%D
%D When scanning a path specification, we also save the
%D operator, using
%D
%D \starttyping
%D \setMPkeyword {n}
%D \stoptyping
%D
%D The path drawing operators are coded for speed: \type{clip},
%D \type{stroke}, \type{fill} and \type{fillstroke} become
%D 1, 2, 3 and~4.
%D
%D When processing the path this code can be retrieved
%D using
%D
%D \starttyping
%D \getMPkeyword % {n}
%D \stoptyping
%D
%D When setting an argument, the exact position on the stack
%D depends on the current value of the \COUNTERS\
%D \type{\nofMPsegments} and \type{\nofMParguments}.

\newcount\nofMPsegments
\newcount\nofMParguments

%D These variables hold the coordinates. The argument part of
%D the stack is reset by:
%D
%D \starttyping
%D \resetMPstack
%D \stoptyping
%D
%D We use the prefix \type{@@MP} to keep the stack from
%D conflicting with existing macros. To speed up things a bit
%D more, we use the constant \type{\@@MP}.

\def\@@MP{@@MP}

\def\setMPargument% #1%
  {\advance\nofMParguments 1
   \expandafter\def
     \csname\@@MP\the\nofMPsegments\the\nofMParguments\endcsname} % {#1}

\def\letMPargument
  {\advance\nofMParguments 1
   \expandafter\let
     \csname\@@MP\the\nofMPsegments\the\nofMParguments\endcsname}

\def\setMPsequence#1 %
  {\advance\nofMParguments 1
   \expandafter\def
     \csname\@@MP\the\nofMPsegments\the\nofMParguments\endcsname{#1}%
   \handleMPsequence}

\def\gMPa#1%
  {\csname\@@MP0\number#1\endcsname}

\def\gMPs#1%
  {\csname\@@MP\the\nofMPsegments\number#1\endcsname}

\def\dogMPa#1%
  {\expandafter\expandafter\expandafter\do\csname\@@MP0\number#1\endcsname}

\def\setMPkeyword#1 %
  {\expandafter\def\csname\@@MP\the\nofMPsegments0\endcsname{#1}%
   \advance\nofMPsegments 1
   \nofMParguments0}

\def\getMPkeyword% #1%
  {\csname\@@MP\the\nofMPsegments0\endcsname} % {\csname\@@MP#10\endcsname}

\def\docleanupMPargument#1% we need this because args can have [ or ] pre/appended
  {\expandafter\edef\csname\@@MP\the\nofMPsegments\number#1\endcsname
     {\csname\@@MP\the\nofMPsegments\number#1\endcsname}}

%D When we reset the stack, we can assume that all further
%D comment is to be ignored and handled in strings.
%D By redefining the reset macro after the first call, we
%D save some run time. Only use this macro after all
%D comments are processed and use the simple alternative
%D when dealing with comments.

\def\doresetMPstack
  {\nofMParguments0\relax}

\def\resetMPstack
  {\let\handleMPgraphic\handleMPendgraphic
   \let\resetMPstack\doresetMPstack
   \resetMPstack}

%D The arguments are saved with the preceding command
%D \type{\do}. By default this command expands to nothing, but
%D when we deal with strings it's used to strip off the
%D \type{(} and \type{)}.
%D
%D Strings are kind of tricky, because characters can be
%D passed verbatim \type{(hello)}, by octal number
%D \type{(\005)} or as command \type{(\()}. We therefore
%D cannot simply ignore \type{(} and \type{)}, the way we do
%D with \type{[} and \type{]}. Another complication is that
%D strings may contain characters that normally have a
%D special meaning in \TEX, like \type{$} and \type{{}}.
%D
%D A previous solution made \type{\} an active character and
%D let it look ahead for a number or characters. We had to
%D abandon this scheme because of the need for verbatim
%D support. The next solution involved some \CATCODE\
%D trickery but works well.

\def\octalMPcharacter#1#2#3%
  {\char'#1#2#3\relax}

%D curly braces and squarly brackets are stored in the argument stack
%D as part  of strings, for instance in:
%D
%D \starttyping
%D /fshow {exch findfont exch scalefont setfont show}bind def
%D [3 3 ] 0 setdash
%D \stoptyping
%D
%D but we need to keep them in situation like
%D
%D \starttyping
%D ([bla bla] bla bla) ec-lmr10 9.96265 fshow
%D ({bla bla} bla bla) ec-lmr10 9.96265 fshow
%D \stoptyping
%D
%D So, when we store the snippets, we keep the special tokens, and
%D when needed we either ignore or obey them

\bgroup
\defineMPtoPDFfallbacks
\catcode`\|=\@@comment
\catcode`\%=\@@active
\catcode`\[=\@@active
\catcode`\]=\@@active
\catcode`\{=\@@active
\catcode`\}=\@@active
\catcode`B=\@@begingroup
\catcode`E=\@@endgroup
\gdef\keepMPspecials|
  B\let%\letterpercent|
   \def[B\noexpand[E|
   \def]B\noexpand]E|
   \def{B\noexpand{E|
   \def}B\noexpand}EE
\gdef\ignoreMPspecials|
  B\let%\letterpercent|
   \def[BE|
   \def]BE|
   \def{BE|
   \def}BEE
\gdef\obeyMPspecials|
  B\def%B\char 37\relax E|
   \def[B\char 91\relax E|
   \def]B\char 93\relax E|
   \def{B\char123\relax E|
   \def}B\char125\relax EE
\gdef\setMPspecials|
  B\setnaturalcatcodes
   \catcode`\\=\@@escape
   \catcode`\%=\@@active
   \catcode`\[=\@@active
   \catcode`\]=\@@active
   \catcode`\{=\@@active
   \catcode`\}=\@@active
   \lccode`\-=0 | latex sets this to `\-
   \lccode`\%=`\% | otherwise it's seen as a number
   \def\(B\char40\relax     E|
   \def\)B\char41\relax     E|
   \def\\B\char92\relax     E|
   \def\0B\octalMPcharacter0E|
   \def\1B\octalMPcharacter1E|
   \def\2B\octalMPcharacter2E|
   \def\3B\octalMPcharacter3E|
   \def\4B\octalMPcharacter4E|
   \def\5B\octalMPcharacter5E|
   \def\6B\octalMPcharacter6E|
   \def\7B\octalMPcharacter7E|
   \def\8B\octalMPcharacter8E|
   \def\9B\octalMPcharacter9EE
\egroup

%D We use the comment symbol as a sort of trigger. Beware!
%D The whole graphic is seen as on eparagraph, which means
%D that we cannot change the catcodes in between.

\bgroup
\defineMPtoPDFfallbacks
\catcode`\%=\@@active
\gdef\startMPscanning{\let%=\startMPconversion}
\egroup

%D In earlier versions we used the sequence
%D
%D \starttyping
%D \expandafter\handleMPsequence\input filename\relax
%D \stoptyping
%D
%D Persistent problems in \LATEX\ however forced us to use a
%D different scheme. Every \POSTSCRIPT\ file starts with a
%D \type{%}, so we temporary make this an active character
%D that starts the scanning and redefines itself. (The problem
%D originates in the redefinition by \LATEX\ of the
%D \type{\input} primitive.)

\def\startMPconversion
  {\keepMPspecials
   \handleMPsequence}

%D Here comes the main loop. Most arguments are numbers. This
%D means that they can be recognized by their \type{\lccode}.
%D This method saves a lot of processing time. We could
%D speed up the conversion by handling the \type{path}
%D seperately.

\def\dohandleMPsequence#1%
  {\ifdone
     \ifcase\lccode`#1\relax
       \expandafter\expandafter\expandafter\dohandleMPsequenceA
     \else
       \expandafter\expandafter\expandafter\dohandleMPsequenceB
     \fi
   \else
     \expandafter\dohandleMPsequenceC
   \fi#1}

\let\dohandleMPsequenceA\setMPsequence

\def\installMPSkeywordN#1#2%
  {\expandafter\def\csname\@@MP:N:#1\endcsname{#2}}

\def\installMPSshortcutN#1#2% todo: \let
  {\expandafter\let\csname\@@MP:N:#1\expandafter\endcsname\csname\@@MP:N:#2\endcsname}

\def\dohandleMPsequenceB#1 %
  {\edef\somestring{#1}%
   \ifcsname\@@MP:N:\somestring\endcsname
     \csname\@@MP:N:\somestring\expandafter\endcsname
   \else
     \expandafter\handleMPgraphic
   \fi
   \handleMPsequence}

\ifx\eTeXversion\undefined
    \def\dohandleMPsequenceB#1 %
      {\edef\somestring{#1}%
       \expandafter\ifx\csname\@@MP:N:\somestring\endcsname\relax
         \expandafter\handleMPgraphic
       \else
         \csname\@@MP:N:\somestring\expandafter\endcsname
       \fi
       \handleMPsequence}
\fi

\installMPSkeywordN \PSmoveto
  {\edef\lastMPmoveX{\gMPa1}%
   \edef\lastMPmoveY{\gMPa2}%
   \resetMPstack}
\installMPSkeywordN \PSnewpath
  {\let\handleMPsequence\handleMPpath}
\installMPSkeywordN \PSgsave
  {\PDFcode{q}%
   \resetMPstack}
\installMPSkeywordN \PSgrestore
  {\PDFcode{Q}%
   \resetMPstack}
\installMPSkeywordN \PSdtransform  % == setlinewidth
  {\let\handleMPsequence\handleMPdtransform}
   % after that we will encounter more tokens until setlinewidth+pop
   % or pop+setlinewidth which we catch next; we explicitly need to
   % reset the stack since [] n setdash may follow; a more clever
   % approach would be to read on till the condition is met, but it's
   % the only pop / setlinewidth we will encounter so ...
\installMPSkeywordN \PSsetlinewidth
  {% already handled in dtransform
   \resetMPstack}
\installMPSkeywordN \PSpop
  {% already handled in dtransform
   \resetMPstack}
\installMPSkeywordN \PSconcat
  {\cleanupMPconcat
   \PDFcode{\gMPa1 \gMPa2 \gMPa3 \gMPa4 \gMPa5 \gMPa6 cm}%
   \resetMPstack}
\installMPSkeywordN \PSsetrgbcolor
  {\handleMPrgbcolor
   \resetMPstack}
\installMPSkeywordN \PSsetcmykcolor
  {\handleMPcmykcolor
   \resetMPstack}
\installMPSkeywordN \PSsetgray
  {\handleMPgraycolor
   \resetMPstack}
\installMPSkeywordN \PStranslate
  {\PDFcode{1 0 0 1 \gMPa1 \gMPa2 cm}%
   \resetMPstack}
\installMPSkeywordN \PSsetdash
  {\handleMPsetdash
   \resetMPstack}
\installMPSkeywordN \PSsetlinejoin
  {\PDFcode{\gMPa1 j}%
   \resetMPstack}
\installMPSkeywordN \PSsetmiterlimit
  {\PDFcode{\gMPa1 M}%
   \resetMPstack}
\installMPSkeywordN \PSfshow
  {%\PDFcode{n}% removed !
   \handleMPfshow
   \resetMPstack}
\installMPSkeywordN \PSsetlinecap
  {\PDFcode{\gMPa1 J}%
   \resetMPstack}
\installMPSkeywordN \PSrlineto
  {\flushMPmoveto
   \PDFcode{\!MP\lastMPmoveX\space\!MP\lastMPmoveY\space l S}%
   \resetMPmoveto
   \resetMPstack}
\installMPSkeywordN \PSscale
  {\PDFcode{\gMPa1 0 0 \gMPa2 0 0 cm}%
   \resetMPstack}
\installMPSkeywordN \PSspecial
  {\handleMPspecialcommand
   \resetMPstack}

\installMPSshortcutN {n}  \PSnewpath
\installMPSshortcutN {p}  \PSclosepath
\installMPSshortcutN {l}  \PSlineto
\installMPSshortcutN {r}  \PSrlineto
\installMPSshortcutN {m}  \PSmoveto
\installMPSshortcutN {c}  \PScurveto
\installMPSshortcutN {C}  \PSsetcmykcolor
\installMPSshortcutN {G}  \PSsetgray
\installMPSshortcutN {R}  \PSsetrgbcolor
\installMPSshortcutN {lj} \PSsetlinejoin
\installMPSshortcutN {ml} \PSsetmiterlimit
\installMPSshortcutN {lc} \PSsetlinecap
\installMPSshortcutN {sd} \PSsetdash
\installMPSshortcutN {S}  \PSstroke
\installMPSshortcutN {F}  \PSfill
\installMPSshortcutN {W}  \PSclip

\installMPSshortcutN {q}  \PSgsave
\installMPSshortcutN {Q}  \PSgrestore

\installMPSshortcutN {s}  \PSscale
\installMPSshortcutN {t}  \PSconcat
\installMPSshortcutN {P}  \PSshowpage

\installMPSkeywordN {hlw} {\PDFcode{\gMPa1 w}\resetMPstack}
\installMPSkeywordN {vlw} {\PDFcode{\gMPa1 w}\resetMPstack}
\installMPSkeywordN {rd}  {\PDFcode{[] 0   d}\resetMPstack}

\def\dohandleMPsequenceC#1 %
  {\edef\somestring{#1}%
   \handleMPgraphic % {#1}%
   \handleMPsequence}

%D Since colors are not sensitive to transformations, they
%D are sometimes used for signaling. Therefore, we handle them
%D separately. The next macro can be redefined if needed.

\def\handleMPrgbcolor
  {\PDFcode{\!MPgMPa1 \!MPgMPa2 \!MPgMPa3 rg
            \!MPgMPa1 \!MPgMPa2 \!MPgMPa3 RG}}

\def\handleMPcmykcolor
  {\PDFcode{\!MPgMPa1 \!MPgMPa2 \!MPgMPa3 \!MPgMPa4 k
            \!MPgMPa1 \!MPgMPa2 \!MPgMPa3 \!MPgMPa4 K}}

\def\handleMPgraycolor
  {\PDFcode{\!MPgMPa1 g
            \!MPgMPa1 G}}

\def\handleMPspotcolor
  {\PDFcode{0 g
            0 G}}

%D Beginning and ending the graphics is taken care of by the
%D macro \type{\handleMPgraphic}, which is redefined when
%D the first graphics operator is met.

\def\handleMPendgraphic % #1%
  {\ifx\somestring\PSshowpage
     \let\handleMPsequence\finishMPgraphic
   \else\ifx\somestring\PSEof
     \let\handleMPsequence\finishMPgraphic
   \else
     \letMPargument\somestring % {#1}%
   \fi\fi}

\def\handleMPbegingraphic % #1%
  {\ifx\somestring\PSBoundingBox
     \def\handleMPsequence{\handleMPboundingbox1}%
   \else\ifx\somestring\PSHiResBoundingBox
     \def\handleMPsequence{\handleMPboundingbox2}%
   \else\ifx\somestring\PSExactBoundingBox
     \def\handleMPsequence{\handleMPboundingbox3}%
   \else\ifx\somestring\PSshowpage
     \let\handleMPsequence\finishMPgraphic
   \else\ifx\somestring\PSEof
     \let\handleMPsequence\finishMPgraphic
   \else\ifx\somestring\PSPage
     \let\handleMPsequence\handleMPpage
   \else\ifx\somestring\PSMetaPostSpecials
     \let\handleMPsequence\handleMPspecialscomment
   \else\ifx\somestring\PSMetaPostSpecial
     \let\handleMPsequence\handleMPspecialcomment
   \else\ifx\somestring\PSBeginProlog
     \let\handleMPsequence\handleMPprolog
   \else
     \letMPargument\somestring % {#1}%
   \fi\fi\fi\fi\fi\fi\fi\fi\fi}

\let\handleMPgraphic=\handleMPbegingraphic

%D New: we can best filter the prolog because nowdays it can contain
%D quite some code.

% hm, catcode mess, so we need to tweak %'s catcode here
% \long\expandafter\def\expandafter\handleMPprolog\expandafter#\expandafter1\PSEndProlog%
% but today i'm not in the mood for ugly stuff

\long\def\handleMPprolog#1EndProlog %
  {\doresetMPstack
   \let\handleMPsequence\dohandleMPsequence
   \handleMPsequence}

%D We check for three kind of bounding boxes: the normal one
%D and two high precision ones:
%D
%D \starttyping
%D BoundingBox: llx lly ucx ucy
%D HiResBoundingBox: llx lly ucx ucy
%D ExactBoundingBox: llx lly ucx ucy
%D \stoptyping
%D
%D The original as well as the recalculated dimensions are
%D saved for later use.

\newif\ifskipemptyMPgraphic \skipemptyMPgraphicfalse

\chardef\currentMPboundingbox=0

\def\handleMPboundingbox#1#2 #3 #4 #5
  {\ifnum#1>\currentMPboundingbox
     \xdef\MPllx{#2}\xdef\MPlly{#3}%
     \xdef\MPurx{#4}\xdef\MPury{#5}%
     \dimen0=#2pt
     \dimen0=-\MPxscale\dimen0
     \dimen2=#3pt
     \dimen2=-\MPyscale\dimen2
     \xdef\MPxoffset{\withoutpt\the\dimen0}%
     \xdef\MPyoffset{\withoutpt\the\dimen2}%
     \dimen0=#2bp
     \dimen0=-\dimen0
     \dimen2=#3bp
     \dimen2=-\dimen2
     \advance\dimen0 #4bp
     \dimen0=\MPxscale\dimen0
     \xdef\MPwidth{\the\dimen0}%
     \advance\dimen2 #5bp
     \xdef\MPyshift{\the\dimen2}% unscaled
     \dimen2=\MPyscale\dimen2
     \xdef\MPheight{\the\dimen2}%
     \chardef\currentMPboundingbox#1\relax
   \fi
   \doresetMPstack
   \let\handleMPsequence\dohandleMPsequence
   \let\next\handleMPsequence
   \ifskipemptyMPgraphic
     \ifdim\MPheight=0pt\relax\ifdim\MPwidth=0pt\relax
       \def\next{\endinput\finishMPgraphic}%
     \fi\fi
   \fi
   \next}

%D Unless defined otherwise, we simply ignore specialcomments.

\def\handleMPspecialcomment
  {\doresetMPstack
   \let\handleMPsequence\dohandleMPsequence
   \handleMPsequence}

\let\handleMPspecialscomment\handleMPspecialcomment

%D We use the \type{page} comment as a signal that
%D stackbuilding can be started.

\def\handleMPpage #1 #2
  {\doresetMPstack
   \donetrue
   \let\handleMPsequence\dohandleMPsequence
   \handleMPsequence}

%D The same applies to the special extensions.

\def\handleMPspecialcommand
  {\doresetMPstack
   \let\handleMPsequence\dohandleMPsequence
   \handleMPsequence}

%D \METAPOST\ draws its dots by moving to a location and
%D invoking \type{0 0 rlineto}. This operator is not
%D available in \PDF. Our solution is straightforward: we draw
%D a line from $(current\_x, current\_y)$ to itself. This
%D means that the arguments of the preceding \type{moveto} have
%D to be saved.

\def\lastMPmoveX{0}
\def\lastMPmoveY{0}

%D These saved coordinates are also used when we handle the
%D texts. Text handling proved to be a bit of a nuisance, but
%D finally I saw the light. It proved that we also had to
%D take care of \type{(split arguments)}.

% \def\setMPfshowfont#1#2%
%   {\font\temp=#1\space at #2\relax\temp}

% \startMPcode
%     draw btex Ga toch effe f\kern0ptietsen?{}` etex ;
% \stopMPcode

\newtoks \everyMPshowfont

\def\setMPfshowfont#1#2%
  {\font\temp=#1\space at #2\relax\temp
   \the\everyMPshowfont}

\let\MPfshowcommand\empty

%D The next hackery handles characters one by one. We only support this
%D for the latest greatest \METAPOST\ binaries, the ones that escape
%D problematic chars.

\def\doflushMPtext#1%
  {\edef\!!stringa{#1}%
   \expandafter\dodoflushMPtext\!!stringa\relax}

\def\dodoflushMPtext
  {\afterassignment\dododoflushMPtext\let\nexttoken=}

\def\dododoflushMPtext
  {\ifx\nexttoken\relax
     % done
   \else\ifx\nexttoken\char
     \expandafter\expandafter\expandafter\dodododoflushMPtext
   \else
     {\nexttoken}%
     \expandafter\expandafter\expandafter\dodoflushMPtext
   \fi\fi}

\def\dodododoflushMPtext
  {\afterassignment\dododododoflushMPtext\scratchcounter}

\def\dododododoflushMPtext
 {{\char\scratchcounter}\let\next\dodoflushMPtext}

\def\dohandleMPfshow
  {\bgroup
   \setbox\scratchbox\hbox
     {\obeyMPspecials
      \let\ \relax % mp breaks long lines and appends a \
      \edef\size{\gMPa\nofMParguments}%
      \ifx\size\PSnfont % round font size (to pt)
        \advance\nofMParguments -1
        \expandafter\scratchdimen\gMPa\nofMParguments pt\relax
        \ifdim\scratchdimen<1pt
          \def\size{1pt}%
        \else
          \advance\scratchdimen .5pt
          \def\size##1.##2\relax{\def\size{##1pt}}%
          \expandafter\size\the\scratchdimen\relax
        \fi
      \else
        \edef\size{\size bp}%
      \fi
      \advance\nofMParguments -1
     %\font\temp=\gMPa\nofMParguments\space at \size
      \let\temp\relax % to be sure
      \setMPfshowfont{\gMPa\nofMParguments}\size
      \advance\nofMParguments -1
      \temp
      \MPfshowcommand
        {\ifnum\nofMParguments=1
           \def\do(##1){##1}%
           \doflushMPtext{\dogMPa1}% only latest mp gets this treatment
         \else
           % we need to catch ( a ) (a a a) (\123 \123 \123) etc
           \scratchcounter1
           \def\dodo##1% Andreas Fieger's bug: (\304...)
             {\edef\!!stringa{##1\empty\empty}% and another one: ( 11) -> \ifx 11
              \ifx\!!stringa\MPspacechar\MPspacechar\else\expandafter##1\fi}%
           \def\do(##1{\dodo{##1}}%
           \dogMPa\scratchcounter\MPspacechar
           \let\do\relax
           \loop
             \advance\scratchcounter 1
             \ifnum\scratchcounter<\nofMParguments\relax
               \gMPa\scratchcounter\MPspacechar
           \repeat
           \def\do##1){\dodo{##1}}%
           \dogMPa\scratchcounter
         \fi
         \unskip}}%
   \setbox\scratchbox\hbox
     {\hskip\lastMPmoveX bp\raise\lastMPmoveY bp\box\scratchbox}%
   \ht\scratchbox0pt%
   \dp\scratchbox0pt%
   \wd\scratchbox0pt%
   \box\scratchbox
   \egroup}

\let\handleMPfshow\dohandleMPfshow % so we can overload this one later

%D You could consider the following definition to be the most
%D natural one.

% \def\MPspacechar{\space} % normal case

\def\MPspacechar{\char32\relax} % old solution does not work with math

%D However, the following implementation is more robust, since
%D some fonts have funny visible spaces in the space slot. This
%D gives a mismatch between the space that \METAPOST\ took into
%D account and the \quote {natural} space. This only happens in
%D labels, since \type {btex}||\type {etex} thingies don't have
%D spaces. This phenomena showed up when preparing the
%D \METAFUN\ manual, where Palatino fonts are used. We can
%D safely assume that \METAPOST\ considers \type {\char32} to
%D be the space.

\def\MPspacechar{\setbox\scratchbox\hbox{\char32}\kern\wd\scratchbox}

%D Well, this does not work with math fonts, so:

\def\MPspacechar{\char32\relax}

%D Most operators are just converted and keep their
%D arguments. Dashes however need a bit different treatment,
%D otherwise \PDF\ viewers complain loudly. Another
%D complication is that one argument comes after the \type{]}.
%D When reading the data, we simply ignore the array boundary
%D characters. We save ourselves some redundant newlines and
%D at the same time keep the output readable by packing the
%D literals.

\def\handleMPsetdash
  {\bgroup
   \ignoreMPspecials
   \def\somestring{[}%
   \scratchcounter1
   \loop
     \ifnum\scratchcounter<\nofMParguments
       \edef\somestring{\somestring\space\gMPa\scratchcounter}%
       \advance\scratchcounter 1
   \repeat
   \edef\somestring{\somestring]\gMPa\scratchcounter\space d}%
   \PDFcode{\somestring}%
   \egroup}

%D The \type{setlinewidth} commands looks a bit complicated. There are
%D two alternatives, that result in a similar look in both
%D $x$- and $y$-dorection. As John Hobby says:
%D
%D \startnarrower \switchtobodyfont[ss]
%D \starttyping
%D x 0 dtransform exch truncate exch idtransform pop setlinewidth
%D 0 y dtransform truncate idtransform setlinewidth pop
%D \stoptyping
%D
%D These are just fancy versions of \type{x setlinewidth} and
%D \type{y setlinewidth}. The \type{x 0 ...} form is used if
%D the path is {\em primarily vertical}. It rounds the width
%D so that vertical lines come out an integer number of pixels
%D wide in device space. The \type{0 y ...} form does the same
%D for paths that are {\em primarily horizontal}. The reason
%D why I did this is Knuth insists on getting exactly the
%D widths \TEX\ intends for the horizontal and vertical rules
%D in \type{btex...etex} output. (Note that PostScript scan
%D conversion rules cause a horizontal or vertical line of
%D integer width $n$ in device space to come out $n+1$ pixels
%D wide, regardless of the phase relative to the pixel grid.)
%D \stopnarrower
%D
%D The common operator in these sequences is \type{dtransform},
%D so we can use this one to trigger setting the linewidth.

\def\handleMPdtransform
  {\ifdim\gMPa1 pt>0pt
     \PDFcode{\gMPa1 w}%
     \def\next##1 ##2 ##3 ##4 ##5 ##6 {\handleMPsequence}%
   \else
     \PDFcode{\gMPa2 w}%
     \def\next##1 ##2 ##3 ##4 {\handleMPsequence}%
   \fi
   \let\handleMPsequence\dohandleMPsequence
   \resetMPstack
   \next}

%D The most complicated command is \type{concat}. \METAPOST\
%D applies this operator to \type{stroke}. At that moment the
%D points set by \type{curveto} and \type{moveto}, are already
%D fixed. In \PDF\ however the \type{cm} operator affects the
%D points as well as the pen (stroke). Like more \PDF\
%D operators, \type{cm} is defined in a bit ambiguous way.
%D The only save route for non||circular penshapes, is saving
%D the path, recalculating the points and applying the
%D transformation matrix in such a way that we can be sure
%D that its behavior is well defined. This comes down to
%D inverting the path and applying \type{cm} to that path as
%D well as the pen. This all means that we have to save the
%D path.

%D In \METAPOST\ there are three ways to handle a path $p$:
%D
%D \starttyping
%D draw p;  fill p;  filldraw p;
%D \stoptyping
%D
%D The last case outputs a \type{gsave fill grestore} before
%D \type{stroke}. Handling the path outside the main loops
%D saves about 40\% run time.\footnote{We can save some more by
%D following the \METAPOST\ output routine, but for the moment
%D we keep things simple.} Switching between the main loop and
%D the path loop is done by means of the recursely called
%D macro \type{\handleMPsequence}.

\def\handleMPpath
  {\chardef\finiMPpath0
   \let\closeMPpath\relax
   \let\flushMPpath\flushnormalMPpath
   \resetMPstack
   \nofMPsegments1
   \let\handleMPsequence\dohandleMPpath
   \dohandleMPpath}

%D Most paths are drawn with simple round pens. Therefore we've
%D split up the routine in two.

\def\flushnormalMPsegment
  {\ifcase\getMPkeyword\relax
     \PDFcode{\!MPgMPs1 \!MPgMPs2 l}%
   \or
     \PDFcode{\!MPgMPs1 \!MPgMPs2 \!MPgMPs3 \!MPgMPs4 \!MPgMPs5 \!MPgMPs6 c}%
   \or
     \PDFcode{\!MP\lastMPmoveX\space\!MP\lastMPmoveY\space l}%
   \or
     \edef\lastMPmoveX{\gMPs1}% evt \!MP here
     \edef\lastMPmoveY{\gMPs2}%
     \PDFcode{\!MP\lastMPmoveX\space \!MP\lastMPmoveY\space m}%
   \fi}

\def\flushconcatMPsegment
  {\ifcase\getMPkeyword\relax
     \doMPconcat{\gMPs1}\a{\gMPs2}\b%
     \PDFcode{\!MP\a\space\!MP\b\space l}%
   \or
     \doMPconcat{\gMPs1}\a{\gMPs2}\b%
     \doMPconcat{\gMPs3}\c{\gMPs4}\d%
     \doMPconcat{\gMPs5}\e{\gMPs6}\f%
     \PDFcode{\!MP\a\space\!MP\b\space
              \!MP\c\space\!MP\d\space
              \!MP\e\space\!MP\f\space c}%
   \or
     \bgroup
     \noMPtranslate
     \doMPconcat\lastMPmoveX\a\lastMPmoveY\b%
     \PDFcode{\!MP\a\space\!MP\b\space l S}%
     \egroup
   \or
     \edef\lastMPmoveX{\gMPs1}%
     \edef\lastMPmoveY{\gMPs2}%
     \doMPconcat\lastMPmoveX\a\lastMPmoveY\b%
     \PDFcode{\!MP\a\space\!MP\b\space m}%
   \fi}

% \def\flushnormalMPpath
%   {\scratchcounter\nofMPsegments
%    \nofMPsegments 1
%    \loop
%      \flushnormalMPsegment
%      \advance\nofMPsegments 1
%      \ifnum\nofMPsegments<\scratchcounter
%    \repeat}
%
% \def\flushconcatMPpath
%   {\scratchcounter\nofMPsegments
%    \nofMPsegments 1
%    \loop
%      \flushconcatMPsegment
%      \advance\nofMPsegments 1
%      \ifnum\nofMPsegments<\scratchcounter
%    \repeat}
%
% an alternative is presented below: (no \def assignment)

\def\doflushsomeMPpath
  {\dodoflushsomeMPpath
   \advance\nofMPsegments 1
   \ifnum\nofMPsegments<\scratchcounter
     \expandafter\doflushsomeMPpath
   \fi}

\def\flushsomeMPpath
  {\scratchcounter\nofMPsegments
   \nofMPsegments 1
   \doflushsomeMPpath}

\def\flushnormalMPpath{\let\dodoflushsomeMPpath\flushnormalMPsegment\flushsomeMPpath}

%OLD \def\flushconcatMPpath{\let\dodoflushsomeMPpath\flushconcatMPsegment\flushsomeMPpath}

%NEW pre-calculate 1/D so it needn't be repeated for each control point.

\def\flushconcatMPpath
  {\MPreciprocaldeterminant
   \let\dodoflushsomeMPpath\flushconcatMPsegment\flushsomeMPpath}

%D The transformation of the coordinates is handled by one of
%D the macros Tanmoy posted to the \PDFTEX\ mailing list.
%D I rewrote and optimized the original macro to suit the other
%D macros in this module.
%D
%D \starttyping
%D \doMPconcat {x position} \xresult {y position} \yresult
%D \stoptyping
%D
%D By setting the auxiliary \DIMENSIONS\ \type{\dimen0} upto
%D \type{\dimen10} only once per path, we save over 20\% run
%D time. Some more speed was gained by removing some parameter
%D passing. These macros can be optimized a bit more by using
%D more constants. There is however not much need for further
%D optimization because penshapes usually are round and
%D therefore need no transformation. Nevertheless we move the
%D factor to the outer level and use a bit different \type{pt}
%D removal macro. Although the values represent base points,
%D we converted them to pure points, simply because those can
%D be converted back.

%OLD \mathchardef\MPconcatfactor=256 % beware don't remove spaces before it

%OLD \def\doMPreducedimen#1
%OLD   {\count0\MPconcatfactor
%OLD    \advance\dimen#1 \ifdim\dimen#1>0pt .5\else -.5\fi\count0
%OLD    \divide\dimen#1 \count0\relax}

%OLD % too inaccurate (see old pragma logo)
%OLD
%OLD \def\doMPreducedimen#1
%OLD   {\count0=\MPconcatfactor
%OLD    \divide\dimen#1 \count0\relax}

%OLD \def\doMPreducedimen#1
%OLD   {\advance\dimen#1 \ifdim\dimen#1>0pt .5\else -.5\fi\MPconcatfactor
%OLD    \divide\dimen#1 \MPconcatfactor}

%D The transformation code is rewritten by Daniel H. Luecking who
%D describes his patch as follows:
%D
%D We would like to divide 1 by $X$, but all divisions are integer so
%D for accuracy we want to convert to large integers and make sure the
%D integer quotient has as many significant digits as possible. Thus we
%D need to replace $1/X$ with $M/N$ where $N$ is as large as possible
%D and $M/N$ is as large as possible. Also for simplicity $M$ should be
%D a power of 2. So we make $M = 2^{30}$ \footnote{$2^{31} - 1$ is the
%D largest legal integer. Using it (and simply ignoring the inaccuracy
%D caused by $-1$) turns out to be at least as accurate in all cases,
%D and more accurate in some.} (largest legal power of 2) and adjust
%D $X$ downward (if necessary) to the the range $1-2^{16}$. This gives
%D at least 15 significant binary digits, (almost as accurate as
%D \METAPOST\ for numbers near 1) or almost 5 significant figures
%D (decimal).

\newcount\MPscratchCnt
\newdimen\MPscratchDim % will be assigned global

\def\MPadjustdimen   % sets \MPscratchDim and \MPscratchCnt
  {\MPscratchCnt0
   \doMPadjustdimen}

\def\doMPadjustdimen
  {\ifdim\MPscratchDim>1pt
     \divide\MPscratchDim 2
     \advance\MPscratchCnt 1
     \expandafter\doMPadjustdimen
   \fi}

%OLD \def\doMPexpanddimen#1
%OLD   {\multiply\dimen#1 \MPconcatfactor\relax}

%D DHL: When viewed as an integer, $1 \hbox{pt}=2^{16}$ so $2^{32}/X$
%D is  the right way to do $(1 \hbox{pt})/(X \hbox{pt})$ and get the
%D answer  in points. But we are limited to $2^{30}/X$. However, we
%D actually do  $[ 2^{30} / (X/2^K) ]*2^{2-K}$ where $K$ is the number
%D of halvings it takes to bring $X$ below $1 \hbox{pt}$. If $K$ is 0
%D or 1 we readjust by multiplying by 4 or 2, otherwise by halving
%D $(K-2)$ times \type {\MPscratchCnt} holds the value of $K$ from
%D \type {\MPadjustdimen}.

\def\MPreadjustdimen  % acts on \MPscratchDim and MPscratchCnt
  {\ifcase\MPscratchCnt
     \multiply\scratchdimen 4
   \or
     \multiply\scratchdimen 2
   \else
     \expandafter\doMPreadjustdimen
   \fi}

\def\doMPreadjustdimen
  {\ifnum\MPscratchCnt>2
     \divide\scratchdimen 2
     \advance\MPscratchCnt -1
     \expandafter\doMPreadjustdimen
   \fi}

\def\MPreciprocaldeterminant
  {\scratchdimen\withoutpt\the\dimen0 \dimen6            % s_x*s_y
   \advance\scratchdimen - \withoutpt\the\dimen2 \dimen4 % s_x*s_y - r_x*r_y
   \ifdim\scratchdimen<0pt  % we need a positive dimension
     \scratchdimen-\scratchdimen   % for \MPadjustdimen (?)
     \doMPreciprocal
     \scratchdimen-\scratchdimen
   \else
     \doMPreciprocal
   \fi
   \edef\MPreciprocal{\withoutpt\the\scratchdimen}}

\newcount\MPnumerator \MPnumerator = 1073741824 % 2^{30}

% todo: dimexpr

\def\doMPreciprocal % replace \scratchdimen with its reciprocal
  {\ifdim\scratchdimen=1pt \else
     \MPadjustdimen
     \scratchcounter\MPnumerator
     \divide\scratchcounter\scratchdimen
     \scratchdimen1\scratchcounter % 1 needed !
     \MPreadjustdimen
  \fi}

%OLD \def\presetMPconcat
%OLD  {\dimen 0=\gMPs1pt \doMPreducedimen 0    % r_x
%OLD   \dimen 2=\gMPs2pt \doMPreducedimen 2    % s_x
%OLD   \dimen 4=\gMPs3pt \doMPreducedimen 4    % s_y
%OLD   \dimen 6=\gMPs4pt \doMPreducedimen 6    % r_y
%OLD   \dimen 8=\gMPs5pt \doMPreducedimen 8    % t_x
%OLD   \dimen10=\gMPs6pt \doMPreducedimen10 }  % t_y
%OLD
%OLD \def\presetMPscale
%OLD   {\dimen 0=\gMPs1pt \doMPreducedimen 0
%OLD    \dimen 2=0pt
%OLD    \dimen 4=0pt
%OLD    \dimen 6=\gMPs2pt \doMPreducedimen 6
%OLD    \dimen 8=0pt
%OLD    \dimen10=0pt}

\def\cleanupMPconcat
  {\ignoreMPspecials
   \docleanupMPargument1%
   \docleanupMPargument6%
   \keepMPspecials}

\def\presetMPconcat
  {\dimen 0=\gMPs1pt   % s_x
   \dimen 2=\gMPs2pt   % r_x
   \dimen 4=\gMPs3pt   % r_y
   \dimen 6=\gMPs4pt   % s_y
   \dimen 8=\gMPs5pt   % t_x
   \dimen10=\gMPs6pt}  % t_y

\def\presetMPscale
  {\dimen 0=\gMPs1pt
   \dimen 2=0pt
   \dimen 4=0pt
   \dimen 6=\gMPs2pt
   \dimen 8=0pt
   \dimen10=0pt}

\def\noMPtranslate % use this one grouped
  {\dimen 8=0pt        % t_x
   \dimen10=0pt}       % t_y

%D \starttyping
%D \def\doMPconcat#1#2#3#4%
%D   {\dimen12=#1 pt \doMPreducedimen12 % p_x
%D    \dimen14=#3 pt \doMPreducedimen14 % p_y
%D    %
%D    \dimen16  \dimen 0
%D    \multiply \dimen16  \dimen 6
%D    \dimen20  \dimen 2
%D    \multiply \dimen20  \dimen 4
%D    \advance  \dimen16 -\dimen20
%D    %
%D    \dimen18  \dimen12
%D    \multiply \dimen18  \dimen 6
%D    \dimen20  \dimen14
%D    \multiply \dimen20  \dimen 4
%D    \advance  \dimen18 -\dimen20
%D    \dimen20  \dimen 4
%D    \multiply \dimen20  \dimen10
%D    \advance  \dimen18  \dimen20
%D    \dimen20  \dimen 6
%D    \multiply \dimen20  \dimen 8
%D    \advance  \dimen18 -\dimen20
%D    %
%D    \multiply \dimen12 -\dimen 2
%D    \multiply \dimen14  \dimen 0
%D    \advance  \dimen12  \dimen14
%D    \dimen20  \dimen 2
%D    \multiply \dimen20  \dimen 8
%D    \advance  \dimen12  \dimen20
%D    \dimen20  \dimen 0
%D    \multiply \dimen20  \dimen10
%D    \advance  \dimen12 -\dimen20
%D    %
%D    \doMPreducedimen16
%D    \divide   \dimen18  \dimen16 \doMPexpanddimen18
%D    \divide   \dimen12  \dimen16 \doMPexpanddimen12
%D    %
%D    \edef#2{\withoutpt\the\dimen18}% % p_x^\prime
%D    \edef#4{\withoutpt\the\dimen12}} % p_y^\prime
%D \stoptyping

%D The following optimization resulted from some tests by
%D and email exchanges with Sanjoy Mahajan.
%D
%D \starttyping
%D \def\doMPconcat#1#2#3#4%
%D   {\dimen12=#1 pt \doMPreducedimen12 % p_x
%D    \dimen14=#3 pt \doMPreducedimen14 % p_y
%D    %
%D    \dimen16  \dimen 0
%D    \multiply \dimen16  \dimen 6
%D    \dimen20  \dimen 2
%D    \multiply \dimen20  \dimen 4
%D    \advance  \dimen16 -\dimen20
%D    %
%D    \dimen18  \dimen12
%D    \multiply \dimen18  \dimen 6
%D    \dimen20  \dimen14
%D    \multiply \dimen20  \dimen 4
%D    \advance  \dimen18 -\dimen20
%D    \dimen20  \dimen 4
%D    \multiply \dimen20  \dimen10
%D    \advance  \dimen18  \dimen20
%D    \dimen20  \dimen 6
%D    \multiply \dimen20  \dimen 8
%D    \advance  \dimen18 -\dimen20
%D    %
%D    \multiply \dimen12 -\dimen 2
%D    \multiply \dimen14  \dimen 0
%D    \advance  \dimen12  \dimen14
%D    \dimen20  \dimen 2
%D    \multiply \dimen20  \dimen 8
%D    \advance  \dimen12  \dimen20
%D    \dimen20  \dimen 0
%D    \multiply \dimen20  \dimen10
%D    \advance  \dimen12 -\dimen20
%D    %
%D   %\ifdim\dimen16>1pt % oeps, can be < 1pt too
%D    \ifdim\dimen16=1pt \else
%D      \ifdim\dimen16>\MPconcatfactor pt
%D        \doMPreducedimen16
%D        \divide \dimen18 \dimen16 \doMPexpanddimen18
%D        \divide \dimen12 \dimen16 \doMPexpanddimen12
%D      \else
%D        \divide \dimen18 \dimen16 \doMPexpanddimen18 \doMPexpanddimen18
%D        \divide \dimen12 \dimen16 \doMPexpanddimen12 \doMPexpanddimen12
%D      \fi
%D    \fi
%D    %
%D    \edef#2{\withoutpt\the\dimen18}% % p_x^\prime
%D    \edef#4{\withoutpt\the\dimen12}} % p_y^\prime
%D \stoptyping
%D
%D But, this one is still too inaccurate, so we now have:

% \def\doMPconcat#1#2#3#4%
%   {\dimen12=#1pt % p_x
%    \dimen14=#3pt % p_y
%    %
%    % we should test for >-1024 too, but for the moment take the gamble
%    \chardef\MPfactor1\ifdim\dimen12<1024pt \ifdim\dimen14<1024pt 6\fi\fi
%    %
%    \multiply\dimen12 \MPfactor
%    \multiply\dimen14 \MPfactor
%    %
%    \doMPreducedimen12
%    \doMPreducedimen14
%    %
%    \dimen16  \dimen 0
%    \multiply \dimen16  \dimen 6
%    \dimen20  \dimen 2
%    \multiply \dimen20  \dimen 4
%    \advance  \dimen16 -\dimen20
%    %
%    \dimen18  \dimen12
%    \multiply \dimen18  \dimen 6
%    \dimen20  \dimen14
%    \multiply \dimen20  \dimen 4
%    \advance  \dimen18 -\dimen20
%    \dimen20  \dimen 4
%    \multiply \dimen20  \dimen10
%    \advance  \dimen18  \dimen20
%    \dimen20  \dimen 6
%    \multiply \dimen20  \dimen 8
%    \advance  \dimen18 -\dimen20
%    %
%    \multiply \dimen12 -\dimen 2
%    \multiply \dimen14  \dimen 0
%    \advance  \dimen12  \dimen14
%    \dimen20  \dimen 2
%    \multiply \dimen20  \dimen 8
%    \advance  \dimen12  \dimen20
%    \dimen20  \dimen 0
%    \multiply \dimen20  \dimen10
%    \advance  \dimen12 -\dimen20
%    %
%    \ifdim\dimen16=1pt \else
%      \ifdim\dimen16>\MPconcatfactor pt
%        \doMPreducedimen16
%        \divide \dimen18 \dimen16 \doMPexpanddimen18
%        \divide \dimen12 \dimen16 \doMPexpanddimen12
%      \else
%        \divide \dimen18 \dimen16 \doMPexpanddimen18 \doMPexpanddimen18
%        \divide \dimen12 \dimen16 \doMPexpanddimen12 \doMPexpanddimen12
%      \fi
%    \fi
%    %
%    \divide\dimen18 \MPfactor
%    \divide\dimen12 \MPfactor
%    %
%    \edef#2{\withoutpt\the\dimen18}% % p_x^\prime
%    \edef#4{\withoutpt\the\dimen12}} % p_y^\prime

%D DHL: Ideally, $r_x$, $r_y$, $s_x$, $s_y$ should be in macros, not
%D dimensions (they are scalar quantities after all, not lengths). I
%D suppose the authors decided to do calculations with integer
%D arithmetic instead of using real factors because it's faster.
%D However, the actual macros test slower, possibly because I've
%D omitted three nested loops. In my test files, my approach is more
%D accurate. It is also far simpler and overflow does not seem to be a
%D significant concern. The scale factors written by Metapost are (?)
%D always $<=1$ (it scales coordinates internally) and coordinates are
%D always likely to be less than \type {\maxdimen}.
%D
%D If this should ever cause problems, the scale factors can be reduced.

% \def\doMPconcat#1#2#3#4%
%   {\dimen12=#1pt % p_x % #1pt
%    \dimen14=#3pt % p_y % #3pt
%    \advance\dimen12 -\dimen8  % p_x - t_x
%    \advance\dimen14 -\dimen10 % p_y - t_y
%    \dimen18=\withoutpt\the\dimen6 \dimen12          % s_y(p_x - t_x)
%    \advance\dimen18 -\withoutpt\the\dimen4 \dimen14 %   - r_y(p_y-t_y)
%    \dimen14=\withoutpt\the\dimen0 \dimen14          % s_x(p_y-t_y)
%    \advance\dimen14 -\withoutpt\the\dimen2 \dimen12 %   - r_x(p_x-t_x)
%    % \MPscratchDim contains precomputed 1/D:
%    \dimen18=\withoutpt\the\MPscratchDim \dimen18
%    \dimen14=\withoutpt\the\MPscratchDim \dimen14
%    \edef#2{\withoutpt\the\dimen18}% % p_x^\prime
%    \edef#4{\withoutpt\the\dimen14}} % p_y^\prime

\def\doMPconcat#1#2#3#4%
  {\dimen12=#1pt % p_x % #1pt
   \dimen14=#3pt % p_y % #3pt
   \advance\dimen12 -\dimen8  % p_x - t_x
   \advance\dimen14 -\dimen10 % p_y - t_y
   \dimen18=\withoutpt\the\dimen6 \dimen12          % s_y(p_x - t_x)
   \advance\dimen18 -\withoutpt\the\dimen4 \dimen14 %   - r_y(p_y-t_y)
   \dimen14=\withoutpt\the\dimen0 \dimen14          % s_x(p_y-t_y)
   \advance\dimen14 -\withoutpt\the\dimen2 \dimen12 %   - r_x(p_x-t_x)
   % \MPreciprocal contains precomputed 1/D:
   \dimen18=\MPreciprocal\dimen18
   \dimen14=\MPreciprocal\dimen14
   \edef#2{\withoutpt\the\dimen18}% % p_x^\prime
   \edef#4{\withoutpt\the\dimen14}} % p_y^\prime

% faster but not that often used
%
% \def\doMPconcat#1#2#3#4%
%   {\dimen12\dimexpr#1\points-\dimen 8\relax % p_x-t_x
%    \dimen14\dimexpr#3\points-\dimen10\relax % p_y-t_y
%    \dimen18\dimexpr\withoutpt\the\dimen6\dimen12-\withoutpt\the\dimen4\dimen14\relax % s_y(p_x-t_x)-r_y(p_y-t_y)
%    \dimen14\dimexpr\withoutpt\the\dimen0\dimen14-\withoutpt\the\dimen2\dimen12\relax % s_x(p_y-t_y)-r_x(p_x-t_x)
%    \edef#2{\withoutpt\the\dimexpr\MPreciprocal\dimen18\relax}% % p_x^\prime
%    \edef#4{\withoutpt\the\dimexpr\MPreciprocal\dimen14\relax}} % p_y^\prime

%D One reason for Daniel to write this patch was that at small sizes
%D the accuracy was less than optimal. Here is a test that demonstrates
%D that his alternative is pretty good:
%D
%D \startlinecorrection
%D \startMPcode
%D for i = 5cm,1cm,5mm,1mm,.5mm,.1mm,.01mm :
%D     draw fullcircle scaled i withpen pencircle xscaled (i/10) yscaled (i/20) rotated 45 ;
%D endfor ;
%D \stopMPcode
%D \stoplinecorrection

%D The following explanation of the conversion process was
%D posted to the \PDFTEX\ mailing list by Tanmoy. The original
%D macro was part of a set of macro's that included sinus and
%D cosinus calculations as well as scaling and translating. The
%D \METAPOST\ to \PDF\ conversion however only needs
%D transformation.

%M \start \switchtobodyfont [ss]

%D Given a point $(U_x, U_y)$ in user coordinates, the business
%D of \POSTSCRIPT\ is to convert it to device space. Let us say
%D that the device space coordinates are $(D_x, D_y)$. Then, in
%D \POSTSCRIPT\ $(D_x, D_y)$ can be written in terms of
%D $(U_x, U_y)$ in matrix notation, either as
%D
%D \placeformula
%D   \startformula
%D   \pmatrix{D_x&D_y&1\cr} = \pmatrix{U_x&U_y&1\cr}
%D                            \pmatrix{s_x&r_x&0\cr
%D                                     r_y&s_y&0\cr
%D                                     t_x&t_y&1\cr}
%D   \stopformula
%D
%D or
%D
%D \placeformula
%D   \startformula
%D    \pmatrix{D_x\cr D_y\cr 1} = \pmatrix{s_x&r_y&t_x\cr
%D                                         r_x&s_y&t_y\cr
%D                                         0  &0  &1  \cr}
%D                                \pmatrix{U_x\cr
%D                                         U_y\cr
%D                                         1  \cr}
%D   \stopformula
%D
%D both of which is a shorthand for the same set of equations:
%D
%D \placeformula
%D   \startformula
%D      D_x = s_x U_x + r_y U_y + t_x
%D   \stopformula
%D
%D \placeformula
%D   \startformula
%D      D_y = r_x U_x + s_y U_y + t_y
%D   \stopformula
%D
%D which define what is called an `affine transformation'.
%D
%D \POSTSCRIPT\ represents the `transformation matrix' as a
%D six element matrix instead of a $3\times 3$ array because
%D three of the elements are always~0, 0 and~1. Thus the above
%D transformation is written in postscript as $[s_x\, r_x\,
%D r_y\, s_y\, t_x\, t_y]$. However, when doing any
%D calculations, it is useful to go back to the original
%D matrix notation (whichever: I will use the second) and
%D continue from there.
%D
%D As an example, if the current transformation matrix is
%D $[s_x\, r_x\, r_y\, s_y\, t_x\, t_y]$ and you say \typ{[a b
%D c d e f] concat}, this means:
%D
%D \startnarrower
%D Take the user space coordinates and transform them to an
%D intermediate set of coordinates using array $[a\, b\, c\, d\,
%D e\, f]$ as the transformation matrix.
%D
%D Take the intermediate set of coordinates and change them to
%D device coordinates using array $[s_x\, r_x\, r_y\, s_y\, t_x\, t_y]$
%D as the transformation matrix.
%D \stopnarrower
%D
%D Well, what is the net effect? In matrix notation, it is
%D
%D \placeformula
%D   \startformula
%D     \pmatrix{I_x\cr I_y\cr 1\cr} = \pmatrix{a&c&e\cr
%D                                             b&d&f\cr
%D                                             0&0&1\cr}
%D                                    \pmatrix{U_x\cr
%D                                             U_y\cr
%D                                             1  \cr}
%D   \stopformula
%D
%D \placeformula
%D   \startformula
%D     \pmatrix{D_y\cr D_y\cr 1\cr} = \pmatrix{s_x&r_y&t_x\cr
%D                                             r_x&s_y&t_y\cr
%D                                             0  &0  &1  \cr}
%D                                    \pmatrix{I_x\cr
%D                                             I_y\cr
%D                                             1  \cr}
%D   \stopformula
%D
%D where $(I_x, I_y)$ is the intermediate coordinate.
%D
%D Now, the beauty of the matrix notation is that when there is
%D a chain of such matrix equations, one can always compose
%D them into one matrix equation using the standard matrix
%D composition law. The composite matrix from two matrices can
%D be derived very easily: the element in the $i$\high{th}
%D horizontal row and $j$\high{th} vertical column is
%D calculated by`multiplying' the $i$\high{th} row of the first
%D matrix and the $j$\high{th} column of the second matrix (and
%D summing over the elements). Thus, in the above:
%D
%D \placeformula
%D   \startformula
%D   \pmatrix{D_x\cr D_y\cr 1} = \pmatrix{s_x^\prime&r_y^\prime&t_x^\prime\cr
%D                                        r_x^\prime&s_y^\prime&t_y^\prime\cr
%D                                        0         &0         &0        \cr}
%D                               \pmatrix{U_x\cr
%D                                        U_y\cr
%D                                        1  \cr}
%D   \stopformula
%D
%D with
%D
%D \placeformula
%D   \startformula
%D      \eqalign
%D        {s_x^\prime & = s_x a + r_y b       \cr
%D         r_x^\prime & = r_x a + s_y b       \cr
%D         r_y^\prime & = s_x c + r_y d       \cr
%D         s_y^\prime & = r_x c + s_y d       \cr
%D         t_x^\prime & = s_x e + r_y f + t_x \cr
%D         t_y^\prime & = r_x e + s_y f + t_y \cr}
%D   \stopformula

%D In fact, the same rule is true not only when one is going
%D from user coordinates to device coordinates, but whenever
%D one is composing two `transformations' together
%D (transformations are `associative'). Note that the formula
%D is not symmetric: you have to keep track of which
%D transformation existed before (i.e.\ the equivalent of
%D $[s_x\, r_x\, r_y\, s_y\, t_x\, t_y]$) and which was
%D specified later (i.e.\ the equivalent of $[a\, b\, c\, d\,
%D e\, f]$). Note also that the language can be rather
%D confusing: the one specified later `acts earlier',
%D converting the user space coordinates to intermediate
%D coordinates, which are then acted upon by the pre||existing
%D transformation. The important point is that order of
%D transformation matrices cannot be flipped (transformations
%D are not `commutative').
%D
%D Now what does it mean to move a transformation matrix
%D before a drawing? What it means is that given a point
%D $(P_x, P_y)$ we need a different set of coordinates
%D $(P_x^\prime, P_y^\prime)$ such that if the transformation
%D acts on $(P_x^\prime, P_y^\prime)$, they produce $(P_x,
%D P_y)$. That is we need to solve the set of equations:
%D
%D \placeformula
%D   \startformula
%D     \pmatrix{P_x\cr P_y\cr 1\cr} = \pmatrix{s_x&r_y&t_x\cr
%D                                             r_x&s_y&t_y\cr
%D                                             0  &0  &1  \cr}
%D                                    \pmatrix{P_x^\prime\cr
%D                                             P_y^\prime\cr
%D                                             1         \cr}
%D   \stopformula
%D
%D Again matrix notation comes in handy (i.e. someone has
%D already solved the problem for us): we need the inverse
%D transformation matrix. The inverse transformation matrix can
%D be calculated very easily:
%D
%D \placeformula
%D   \startformula
%D     \pmatrix{P_x^\prime\cr P_y^\prime\cr 1\cr} =
%D        \pmatrix{s_x^\prime&r_y^\prime&t_x^\prime\cr
%D                 r_x^\prime&s_y^\prime&t_y^\prime\cr
%D                 0  &0  &1  \cr}
%D        \pmatrix{P_x\cr
%D                 P_y\cr
%D                 1         \cr}
%D   \stopformula
%D
%D where, the inverse transformation matrix is given by
%D
%D \placeformula
%D   \startformula
%D     \eqalign
%D       {D          & = s_x s_y - r_x r_y           \cr
%D        s_x^\prime & = s_y / D                     \cr
%D        s_y^\prime & = s_x / D                     \cr
%D        r_x^\prime & = - r_x / D                   \cr
%D        r_y^\prime & = - r_y / D                   \cr
%D        t_x^\prime & = ( - s_y t_x + r_y t_y ) / D \cr
%D        t_y^\prime & = (   r_x t_x - s_x t_y ) / D \cr}
%D   \stopformula
%D
%D And you can see that when expanded out, this does
%D give the formulas:
%D
%D \placeformula
%D   \startformula
%D     P_x^\prime = { { s_y(p_x-t_x) + r_y(t_y-p_y) } \over
%D                    { s_x s_y-r_x r_y } }
%D   \stopformula
%D
%D \placeformula
%D   \startformula
%D     P_y^\prime = { { s_x(p_y-t_y) + r_x(t_x-p_x) } \over
%D                    { s_x*s_y-r_x*r_y } }
%D   \stopformula
%D
%D The code works by representing a real number by converting
%D it to a dimension to be put into a \DIMENSION\ register: 2.3 would
%D be represented as 2.3pt for example. In this scheme,
%D multiplying two numbers involves multiplying the \DIMENSION\
%D registers and dividing by 65536. Accuracy demands that the
%D division be done as late as possible, but overflow
%D considerations need early division.
%D
%D Division involves dividing the two \DIMENSION\ registers and
%D multiplying the result by 65536. Again, accuracy would
%D demand that the numerator be multiplied (and|/|or the
%D denominator divided) early: but that can lead to overflow
%D which needs to be avoided.
%D
%D If nothing is known about the numbers to start with (in
%D concat), I have chosen to divide the 65536 as a 256 in each
%D operand. However, in the series calculating the sine and
%D cosine, I know that the terms are small (because I never
%D have an angle greater than 45 degrees), so I chose to
%D apportion the factor in a different way.

%M \stop

%D The path is output using the values saved on the stack. If
%D needed, all coordinates are recalculated.

\def\finishMPpath
  {\PDFcode{\ifcase\finiMPpath W n\or S\or f\or B\fi}}

\def\processMPpath
  {\checkMPpath
   \ifcase\nofMPsegments\else
     \flushMPpath
     \closeMPpath
     \finishMPpath
   \fi
   \let\handleMPsequence\dohandleMPsequence
   \resetMPstack
   \nofMPsegments0
   \handleMPsequence}

%D The following \METAPOST\ code is quite valid but, when
%D processed and converted to \PDF, will make a file
%D unprintable on a Hewlett Packard printer (from Acrobat
%D $v<=5$). Who is to blame, the driver of the OS layer in
%D between, is hard to determine, so we add an additional
%D check.
%D
%D \starttyping
%D clip currentpicture to origin -- cycle ;
%D setbounds currentpicture to fullsquare scaled 5cm ;
%D \stoptyping

\def\checkMPpath
  {\ifcase\finiMPpath
     \ifnum\nofMPsegments<3 % n is one ahead
       \message{omitting zero clip path}%
       \nofMPsegments0
     \fi
   \fi}

%D In \PDF\ the \type{cm} operator must precede the path
%D specification. We therefore can output the \type{cm} at
%D the moment we encounter it.

\def\handleMPpathconcat
  {\presetMPconcat
   \PDFcode{\gMPs1 \gMPs2 \gMPs3 \gMPs4 \gMPs5 \gMPs6 cm}%
   \resetMPstack}

\def\handleMPpathscale
  {\presetMPscale
   \PDFcode{\gMPs1 0 0 \gMPs2 0 0 cm}%
   \resetMPstack}

%D This macro interprets the path and saves it as compact as
%D possible.

\def\dohandleMPpath#1%
  {\ifcase\lccode`#1\relax
     \expandafter\dohandleMPpathA
   \else
     \expandafter\dohandleMPpathB
   \fi#1}

%\def\dohandleMPpathA#1 %
%  {\setMPargument{#1}%
%   \handleMPsequence}

\let\dohandleMPpathA\setMPsequence

% \def\dohandleMPpathB#1 %
%   {\def\somestring{#1}%
%    \ifx\somestring\PSlineto
%      \setMPkeyword0
%    \else\ifx\somestring\PScurveto
%      \setMPkeyword1
%    \else\ifx\somestring\PSrlineto
%      \setMPkeyword2
%    \else\ifx\somestring\PSmoveto
%      \setMPkeyword3
%    \else\ifx\somestring\PSclip
%    % \chardef\finiMPpath0 % already
%      \let\handleMPsequence\processMPpath
%    \else\ifx\somestring\PSgsave
%      \chardef\finiMPpath3
%    \else\ifx\somestring\PSgrestore
%    \else\ifx\somestring\PSfill
%      \ifcase\finiMPpath
%        \chardef\finiMPpath2
%        \let\handleMPsequence\processMPpath
%      \fi
%    \else\ifx\somestring\PSstroke
%      \ifcase\finiMPpath
%        \chardef\finiMPpath1
%      \fi
%      \let\handleMPsequence\processMPpath
%    \else\ifx\somestring\PSclosepath
%      \def\closeMPpath{\PDFcode{h}}%
%    \else\ifx\somestring\PSconcat
%      \cleanupMPconcat
%      \let\flushMPpath\flushconcatMPpath
%      \handleMPpathconcat
%    \else\ifx\somestring\PSscale
%      \let\flushMPpath\flushconcatMPpath
%      \handleMPpathscale
%    \fi\fi\fi\fi\fi\fi\fi\fi\fi\fi\fi\fi
%    \handleMPsequence}

\def\installMPSkeywordP#1#2%
  {\expandafter\def\csname\@@MP:P:#1\endcsname{#2}}

\def\installMPSshortcutP#1#2% todo: \let
  {\expandafter\let\csname\@@MP:P:#1\expandafter\endcsname\csname\@@MP:P:#2\endcsname}

\def\dohandleMPpathB#1 %
  {\def\somestring{#1}%
   \ifcsname\@@MP:P:\somestring\endcsname
     \csname\@@MP:P:\somestring\expandafter\endcsname
   \fi
   \handleMPsequence}

\ifx\eTeXversion\undefined
    \def\dohandleMPpathB#1 %
      {\def\somestring{#1}%
       \csname\@@MP:P:\somestring\endcsname
       \handleMPsequence}
\fi

\installMPSkeywordP \PSlineto
  {\setMPkeyword0 }
\installMPSkeywordP \PScurveto
  {\setMPkeyword1 }
\installMPSkeywordP \PSrlineto
  {\setMPkeyword2 }
\installMPSkeywordP \PSmoveto
  {\edef\lastMPmoveX{\gMPs1}%
   \edef\lastMPmoveY{\gMPs2}%
   \resetMPstack
   \setMPkeyword3 }
\installMPSkeywordP \PSclip
  {% \chardef\finiMPpath\zerocount % already
   \let\handleMPsequence\processMPpath}
\installMPSkeywordP \PSgsave
  {\chardef\finiMPpath3 }
\installMPSkeywordP \PSgrestore
  {}
\installMPSkeywordP \PSfill
  {\ifcase\finiMPpath
     \chardef\finiMPpath2
     \let\handleMPsequence\processMPpath
   \fi}
\installMPSkeywordP \PSstroke
  {\ifcase\finiMPpath
    \chardef\finiMPpath1
   \fi
   \let\handleMPsequence\processMPpath}
\installMPSkeywordP \PSclosepath
  {\def\closeMPpath{\PDFcode{h}}}
\installMPSkeywordP \PSconcat
  {\cleanupMPconcat
   \let\flushMPpath\flushconcatMPpath
   \handleMPpathconcat}
\installMPSkeywordP \PSscale
  {\let\flushMPpath\flushconcatMPpath
   \handleMPpathscale}

\installMPSshortcutP {l} \PSlineto
\installMPSshortcutP {r} \PSrlineto
\installMPSshortcutP {m} \PSmoveto
\installMPSshortcutP {c} \PScurveto

\installMPSshortcutP {q} \PSgsave
\installMPSshortcutP {Q} \PSgrestore
\installMPSshortcutP {S} \PSstroke
\installMPSshortcutP {F} \PSfill
\installMPSshortcutP {B} \PSgsave
\installMPSshortcutP {W} \PSclip
\installMPSshortcutP {p} \PSclosepath

\installMPSshortcutP {s} \PSscale
\installMPSshortcutP {t} \PSconcat

%D The main conversion command is:
%D
%D \starttyping
%D \convertMPtoPDF {filename} {x scale} {y scale}
%D \stoptyping
%D
%D The dimensions are derived from the bounding box. So we
%D only have to say:
%D
%D \starttyping
%D \convertMPtoPDF{mp-pra-1.eps}{1}{1}
%D \convertMPtoPDF{mp-pra-1.eps}{.5}{.5}
%D \stoptyping

%D \macros
%D   {makeMPintoPDFobject,lastPDFMPobject}
%D
%D For experts there are a few more options. When attributes
%D are to be added, the code must be embedded in an object
%D accompanied with the appropriate directives. One can
%D influence this process with \type {\makeMPintoPDFobject}.
%D
%D This option defaults to~0, because \CONTEXT\ takes care
%D of objects at another level, which saves some bytes.
%D
%D \starttabulate[|l|l|p|]
%D \NC 0 \NC never    \NC don't use an object    \NC\NR
%D \NC 1 \NC always   \NC always use an object   \NC\NR
%D \NC 2 \NC optional \NC use object when needed \NC\NR
%D \stoptabulate
%D
%D The last object number used is avaliable in the macro
%D \type {\lastPDFMPobject}.

\ifx\makeMPintoPDFobject\undefined \newcount\makeMPintoPDFobject \fi

\def\lastPDFMPobject{0}

%D The additional code needed can be made available in the
%D (global) macro \type {\currentPDFresources}.

\let\currentPDFresources\empty

\newtoks\everyMPtoPDFconversion

\def\convertMPtoPDF % #1#2#3%
  {\bgroup
   \defineMPtoPDFfallbacks
   \ifx\pdfdecimaldigits\undefined\else \pdfdecimaldigits=5 \fi % new
   \setbox\scratchbox\vbox\bgroup
     \xdef\MPheight{0pt}%
     \xdef\MPwidth {0pt}%
     \forgetall
     \offinterlineskip
     \startMPresources
     \doprocessMPtoPDFfile} %

%D The next one is kind of private and probably will become obsolete):

\def\processMPtoPDFfile % file xscale yscale
  {\bgroup
   \let\finishMPgraphic\egroup
   \doprocessMPtoPDFfile}

\let\setMPextensions\relax

\def\doprocessMPtoPDFfile#1#2#3% file xscale yscale
  {\setMPspecials
   \setMPextensions
   \the\everyMPtoPDFconversion
   \catcode`\^^M=\@@endofline
   \startMPscanning
   \let\do\empty
   \xdef\MPxscale{#2}%
   \xdef\MPyscale{#3}%
   \xdef\MPxoffset{0}%
   \xdef\MPyoffset{0}%
   \xdef\MPyshift{0pt}%
   \donefalse
   \let\handleMPsequence\dohandleMPsequence
   \message{[MP to PDF]}% was: [MP to PDF #1] but there is a (#1) anyway
   \input#1\relax}

\def\PDFMPformoffset
  {\ifx\objectoffset\undefined0pt\else\objectoffset\fi}

\chardef\blackoutMPgraphic0 % in ConTeXt 1

\def\finishMPgraphic
  {\stopMPresources
   \egroup
   \setbox\scratchbox\vbox
     {\forgetall
      \hbox
        {\PDFcode{q \MPxscale\space 0 0 \MPyscale\space \MPxoffset\space \MPyoffset\space cm}%
         \ifcase\blackoutMPgraphic\or\PDFcode{0 g 0 G}\fi
         \lower\MPyshift\box\scratchbox % unscaled shift
         \PDFcode{Q}}}%
   \ht\scratchbox\MPheight
   \wd\scratchbox\MPwidth
   \dp\scratchbox0pt\relax
   \dopackageMPgraphic\scratchbox
   \egroup
   \endinput}

%D Alternative for \PDFTEX. We cannot come up with something more contexy
%D because this module is also used in \LATEX.

\def\dopackageMPgraphic#1% #1 = boxregister
  {%\ifx\pdfxform\undefined
   %  \makeMPintoPDFobject0 % no pdftex at all
   %\else\ifx\pdftexversion\undefined
   %  \makeMPintoPDFobject0 % no pdftex at all
   %\else\ifnum\pdftexversion<14
   %  \makeMPintoPDFobject0 % no resource support
   %\else
   %                                         % keep the default value
   %\fi\fi\fi
   \ifcase\makeMPintoPDFobject\or\or\ifx\currentPDFresources\empty\else
     % an existing value of 2 signals object support (set elsewhere)
     \makeMPintoPDFobject1
   \fi\fi
   \ifcase\makeMPintoPDFobject
     \box#1%
   \or
     \scratchdimen\PDFMPformoffset\relax
     \ifdim\scratchdimen>0pt % compensate for error
       \setbox#1\vbox spread 2\scratchdimen
         {\forgetall\vss\hbox spread 2\scratchdimen{\hss\box#1\hss}\vss}%
     \fi
     \setMPPDFobject{\currentPDFresources}{#1}%
     \ifdim\scratchdimen>0pt % compensate for error
       \vbox to \MPheight
         {\forgetall\vss\hbox to \MPwidth{\hss\getMPPDFobject\hss}\vss}%
     \else
       \getMPPDFobject
     \fi
     \global\let\currentPDFresources\empty
   \else
     \box#1%
   \fi}

\def\setMPPDFobject#1#2% resources boxnumber
  {\ifx\pdfxform\undefined
     \def\getMPPDFobject{\box#2}%
   \else\ifx\pdftexversion\undefined
     \def\getMPPDFobject{\box#2}%
   \else\ifnum\pdftexversion<14
     \def\getMPPDFobject{\box#2}%
   \else
     \ifx\everyPDFxform\undefined\else\the\everyPDFxform\fi
     \immediate\pdfxform resources{#1}#2%
     \edef\getMPPDFobject{\noexpand\pdfrefxform\the\pdflastxform}%
   \fi\fi\fi}

\let\getMPPDFobject\relax

%D \macros
%D   {deleteMPgraphic,
%D    startMPresources,
%D    stopMPresources}
%D
%D Here are a few hooks for \CONTEXT\ specific things.

\ifx\deleteMPgraphic\undefined
  \def\deleteMPgraphic#1{}
\fi

\ifx\startMPresources\undefined
  \let\startMPresources\relax
  \let\stopMPresources\relax
\fi

%D \macros
%D   {twodigitMPoutput}
%D
%D We can limit the precision to two digits after the comma
%D by saying:
%D
%D \starttyping
%D \twodigitMPoutput
%D \stoptyping
%D
%D This option only works in \CONTEXT\ combined with \ETEX.

\def\twodigitMPoutput
  {\let\!MP        \twodigitrounding
   \def\!MPgMPs##1{\twodigitrounding{\gMPs##1}}%
   \def\!MPgMPa##1{\twodigitrounding{\gMPa##1}}}

\let\!MP    \empty
\let\!MPgMPa\gMPa
\let\!MPgMPs\gMPs

%D This kind of conversion is possible because \METAPOST\
%D does all the calculations. Converting other \POSTSCRIPT\
%D files would drive both me and \TEX\ crazy.

\protect \endinput
